# Supplementary material for: Real-time dense 3D Reconstruction from monocular video data captured by low-cost UAVs
Source: arXiv:2104.10515 source file (2021-04-21)
Supplement: Supplementary file 1 [file 08_appendix.tex]

\section*{APPENDIX (Optional)}\label{Asec:appendix}

Any additional supporting data may be appended, provided the paper does not exceed the limits given above.
